# Supplementary material for: The reverse mathematics of the Thin set and Erd\H{o}s-Moser theorems
Source: arXiv:2103.07880 source file (2021-11-16)
Supplement: Supplementary file 1 [file appendix.tex]

We design a property that is not preserved by
$\msf{SEM}$ but is preserved by
$\msf{WKL},\msf{COH},\msf{FS}^2,\msf{TS}^2_4$.
The property is as following.

\begin{definition}

A collection of finite set pair
$\t{E}_n,\t{F}_n,n\in\omega$
is C-\hyper\ if  for every
C-computable collection of finite sets
$E_n,F_{n,m},n,m\in\omega$ with
$E_n>n\wedge F_{n,m}>m$, there exists
$n,m,n'$ such that
$E_n\subseteq \t{E}_{n'}\wedge
F_{n,m}\subseteq \t{F}_{n'}$.

\end{definition}

\begin{definition}
Problem $\msf{P}$ \emph{preserves} \propertyL\ if
for every  collection of finite set pair
$\EF$ that is $C$-\hyper,
every $C$-computable $\msf{P}$-instance
admit a solution $G$ such that
$\EF$ is $C\oplus G$-\hyper.

Problem $\msf{P}$ \emph{strongly preserves} \propertyL\ if
for every  collection of finite set pair
$\EF$ that is $C$-\hyper,
every $\msf{P}$-instance
admit a solution $G$ such that
$\EF$ is $C\oplus G$-\hyper.
\end{definition}

\begin{theorem}\label{TSth1}
$\mathsf{EM}$, $\msf{SADS}$
do not preserve \propertyL.
\end{theorem}

The proof is given in section \ref{TSsec1}.

\begin{theorem}\label{TSth2}
$\msf{WKL},\msf{COH}$
preserve \propertyL.
\end{theorem}
The proof is given in section \ref{TSsec2}.

\begin{theorem}\label{TSth3}
$\msf{FS}^2,\msf{TS}^2_4$ preserve \propertyL.
\end{theorem}
The proof is given after theorem \ref{TSth4}.
The following corollary follows directly from theorem
\ref{TSth2},\ref{TSth3}.
\begin{corollary}
Over $\msf{RCA}_0$,
$\msf{WKL}+\msf{COH}+\msf{FS}^2+\msf{TS}^2_4$
implies neither $\msf{SEM}$
nor $\msf{SADS}$.
\end{corollary}
\begin{proof}
By theorem \ref{TSth1},
for some collection of set pairs
$\EF$ that is \hyper, there exists a computable
$\msf{SEM}$ instance $\mcal{T}$ such that for every
infinite transitive subtournament $H$ of $\mcal{T}$, $H$
 compute
a collection of finite sets  $E_n,F_{n,m}$ with
$E_n>n\wedge F_{n,m}>m$ and $(\forall n,m,n')
[E_n\subseteq \t{E}_{n'}\rightarrow
F_{n,m}\nsubseteq \t{F}_{n'}]$.
Meanwhile, by theorem \ref{TSth2},
\ref{TSth3} there exists a model
of $\msf{WKL}+\msf{COH}+\msf{TS}_4^2+\msf{FS}^2$
such that for every set $G$ in this model,
$\EF$ is $G-$\hyper. Therefore this model
does not contain an infinite subtournament of $\mcal{T}$
and is not a model of $\msf{RCA}_0+\msf{SEM}$.
For more information on how to use
property preservation to separate theorems,
see also \cite{}.
\end{proof}

To prove theorem \ref{TSth3} we apply the
CJS (\cite{})
 decomposition for $\msf{TS}_4^2$ and $\msf{FS}^2$.

\begin{theorem}\label{TSth4}
$\msf{TS}_4^1$,
$\msf{LFS^1}$ and
$\msf{UFS}^2$ strongly preserve
\propertyL.
\end{theorem}
The proof is given in section \ref{TSsec3},\ref{TSsec4},
\ref{TSsec5}.
\begin{proof}[Proof of theorem \ref{TSth3}]
Note that $\msf{TS}_4^2$ follows from
$\msf{COH}+\msf{STS}_4^2$. Meanwhile,
for every $\msf{STS}_4^2$
instance $c$, $c\oplus H$ compute
an infinite thin set of $c$, where
$H$ is any infinite thin set of the following
$\msf{TS}_4^1$ instance:
$\t{c}(x) = k$ if and only if
$c(\{x,y\}) = k$ for all but finitely many $y$.
But $\msf{TS}_4^1$ strongly preserves
\propertyL. So $\msf{STS}_4^2$ preserves
\propertyL. Therefore
$\msf{TS}_4^2$ preserves \propertyL\ 
 as well.

 To prove $\msf{FS}^2$ preserve \propertyL,
observe that a free set of a $\msf{FS}^2$
instance $c$ can be
obtained by invoking computable instance of
$\msf{COH}$, a (non computable) $\msf{UFS}^2$ and a
(non computable)
 $\msf{LFS}^1$ instance in the following way.
Firstly invoke a computable instance of
$\msf{COH}$, $\vec{R}=(R_1,R_2,\cdots)$, such that
 $c$ is
stable restricted on every $\vec{R}$-cohesive set.
 Suppose $X$ is an infinite
$\vec{R}$-cohesive set. Consider the following
 $\msf{UFS}^2,\msf{LFS}^1$ instance:
for any $x<y\in X$,
\begin{align}
&c_U(\{x,y\}) =\left\{
\begin{aligned}
& c(\{x,y\})
\ \ \text{ if } c(\{x,y\})>x;\\
& y \hspace{1.5cm} \text{ if else.}
\end{aligned}
\right.
\\
&c_L(x) =\left\{
\begin{aligned}
& z
\ \ \ \text{ if for all but finitely many }y,
c(\{x,y\})=z\leq x;\\
& x  \ \ \ \text{ if else.}
\end{aligned}
\right.
\end{align}
Let $Z\subseteq X$ be any infinite free set of both
$c_L,c_U$.
Clearly, for any $x\in Z$,
$c(\{x,y\})\in \{x,y\}\vee
c(\{x,y\})\notin Z$ for all but finitely many
$y$. Thus it is plain to see that
$c\oplus Z$ compute an infinite free set of $c$.
Thus $\msf{FS}^2$ preserve \propertyL\ since
by theorem \ref{TSth2} $\msf{COH}$ preserve \propertyL\ 
and
 by theorem \ref{TSth4}, $\msf{LFS^1}$
 and
$\msf{UFS}^2$ strongly preserve
\propertyL.

\end{proof}

We give proofs of theorem\ref{TSth1},
\ref{TSth2}, \ref{TSth4} in the following sections.
The proof for preservation of \propertyL\ 
follows the traditional method of Seetapun\cite{}
(but with different combinatorics other than partitions).
In the following text we fix a collection of finite set pair
$\EF$ that is \hyper.
For notation convenience we regard each
Turing machine $\Phi$ as computing
some collection of finite set pair,
 $E_n = \Phi(n;1),F_{n,m} = \Phi(n,m;2)$.

\subsection{$\msf{TS}_4^1$ strongly preserve \propertyL}
\label{TSsec3}
We prove that every $\msf{TS}_4^1$ instance
admit an infinite thin set $G $ such that $\EF$ is
$G$-\hyper. This suffices for our purpose
since our result relativizes.

\subsubsection{Requirements}
Fix a $\msf{TS}_4^1$ instance $\vec{A}
=A_1\oplus A_2\oplus A_3\oplus A_4$
where $A_1\oplus A_2\oplus A_3\oplus A_4$ is a
4-partition of $\omega$.
we construct $G$ such that
$\EF$ is $G\cap A_i^c$-\hyper\ 
and $G\cap A_i^c$ is infinite for some $i\in\{1,2,3,4\}$.
The requirements we use is simply for each tuple 
$(e_1,e_2,e_3)\in\omega^3$:
$$
\mcal{R}^1_{e_1}\vee \mcal{R}^2_{e_2}\vee
\mcal{R}^3_{e_3}\vee \mcal{R}^4_{e_4},
$$
where $\mcal{R}^i_e$ says that if $\Phi_e^{G\cap A^c_i}$
is total, then
there exists $n,m,n'$ such that either
$\Phi_e^{G\cap A^c_i}(n;1)\ngtr n\vee
\Phi_e^{G\cap A^c_i}(n,m;2)\ngtr m$  or
$\Phi_e^{G\cap A^c_i}(n;1)\subseteq \t{E}_{n'}\wedge
\Phi_e^{G\cap A^c_i}(n,m;2)\subseteq \t{F}_{n'}$. i.e.,
\begin{align}
\mcal{R}^i_e:
(\exists n,m,n')\ \bigg[
&\Phi_e^{G\cap A_i^c}(n;1)\uparrow\vee
\Phi_e^{G\cap A_i^c}(n;1)\downarrow\ngtr n
\\ \nonumber
&\vee
\Phi_e^{G\cap A_i^c}(n,m;2)\uparrow\vee
\Phi_e^{G\cap A_i^c}(n,m;2)\downarrow\ngtr m
\\ \nonumber
&\vee
\big(\Phi_e^{G\cap A_i^c}(n;1)\downarrow
\subseteq \t{E}_{n'},
\Phi_e^{G\cap A_i^c}(n,m;2)\downarrow
\subseteq \t{F}_{n'}
\big)
\ \
\bigg].
\end{align}
%If $\Phi(n,j;2)\uparrow$ we regard it as an empty set.
%Note that the requirements we use
%are actually stronger than what we need.
The positive requirements are
for every $e\in\omega$:
$$\mcal{P}^i_{e}: \#G\cap A_i^c >e.$$
If $G $ satisfy
all requirements
$\mcal{P}^i_e,i\in\{1,2,3,4\},e\in\omega$,
then clearly
each of $G\cap A_{1}^c,G\cap A_{2}^c,
G\cap A_3^c, G\cap A_4^c$ is infinite.
If $G$ satisfy all requirements
$\mcal{R}^1_{e_1}\vee \mcal{R}^2_{e_2}\vee
\mcal{R}^3_{e_3}\vee \mcal{R}^4_{e_4},e_1,e_2,e_3,
e_4\in\omega$
then for some $i\in\{1,2,3,4\}$,
$G$ satisfy all $\mcal{R}^i_e,e\in\omega$.
Thus  $\EF$ is $G\cap A_i^c$-\hyper.

\subsubsection{Forcing condition}
\label{TSsubsec3}
The forcing condition in this section
is Mathias condition
 $(\sigma,X)$.
In this section, we say a condition
$(\sigma,X)$ is \emph{valid} if:
$X$ is infinite and
 $\EF$ is $X$-\hyper.
In this section, a condition
$(\sigma,X)$ is \emph{positive}
if each of $X\cap A_1^c,X\cap A_2^c,X\cap A_3^c,
X\cap A_4^c$
is infinite.
Every forcing condition in this paper is
essentially a collection of sets
(more precisely, closed set).
For a Mathias forcing condition
$(\sigma,X)$, the collection of sets
of $(\sigma,X)$
refers to
$\{Y/\sigma:Y\subseteq X \}$.
Here and below, we say a condition $d$ forces
a requirement $\mcal{R}$ if every
set in $d$ satisfy requirement $\mcal{R}$.
Condition $d_1$ \emph{extends}
condition $d_2$, denoted as $d_1\leq d_2$,
if $d_1$ as a collection of sets is
a sub collection of $d_2$.

\subsubsection{Framework of proof}
\label{TSsubsec2}
\begin{lemma}\label{TSlem1}
For every valid condition
$(\sigma,X)$, every
requirement
$\mcal{R}^1_{e_1}\vee \mcal{R}^2_{e_2}\vee
\mcal{R}^3_{e_3}\vee\mcal{R}^4_{e_4}$ there exists
a valid condition
$(\rho, Y)\leq (\sigma,X)$ that forces
$\mcal{R}^1_{e_1}\vee \mcal{R}^2_{e_2}\vee
\mcal{R}^3_{e_3}\vee\mcal{R}^4_{e_4}$.

\end{lemma}
The proof of this key
lemma is delayed to section \ref{TSsubsec1}.

\begin{lemma}\label{TSlem2}
If a valid condition $(\sigma,X)$ does not have an
extension satisfying a given positive requirement
$\mcal{P}^i_e$, then
 $\EF$ is $X\cap A_i$-\hyper.
Therefore let $G=X\cap A_i$, then $G$ is an infinite
thin set of $A$ and  $\EF$ is $G$-\hyper.
\end{lemma}
\begin{proof}
This is trivial. If
$(\sigma,X)$ can not be extended
to satisfy $\mcal{P}^i_e$, then
$X\cap A_i^c$ must be finite. Thus
$X\cap A_i$ is co-finite.
Therefore $\EF$ is $X\cap A_i$-\hyper
 since $X\cap A_i\leq _T X$ and
$\EF$ is $X$-\hyper.
\end{proof}

Now assuming lemma \ref{TSlem1},\ref{TSlem2},
we construct the desired $G$.
By lemma \ref{TSlem1},\ref{TSlem2},
construct a sequence of valid forcing condition
$d_0\geq d_1\geq \cdots$ such that
$d_0 = (\varepsilon, \omega)$,
$d_{2<e_1,e_2,e_3,e_4>}$ forces
$\mcal{R}^1_{e_1}\vee \mcal{R}^2_{e_2}\vee
\mcal{R}^3_{e_3}\vee\mcal{R}^4_{e_4}$ and
$d_{2<e,i>+1}$ forces $\mcal{P}_e^i$.
If such a sequence does not exists, it must be
the case that for some
valid forcing condition $d_s$,
$d_s= (\sigma^s,X^s)$ does not have an
extension satisfying some positive requirement
$\mcal{P}^i_e$. Therefore by lemma \ref{TSlem2}
the desired $G$ can be simply $X^s\cap A_i$.
If such a sequence exists, then
$G=\bigcup\limits_{s}\sigma^s$ is an element of every
$d_s$. Thus this $G$ satisfies
all requirements
$\mcal{P}^i_e,i\in\{1,2,3,4\},e\in\omega$
and
$\mcal{R}^1_{e_1}\vee \mcal{R}^2_{e_2}\vee
\mcal{R}^3_{e_3}\vee\mcal{R}^4_{e_4},e_1,e_2,e_3,e_4\in\omega$.
\subsubsection{Proof of lemma \ref{TSlem1}}
\label{TSsubsec1}
Fix a valid condition $(\sigma,X)$,
and a requirement $\mcal{R}^1_{e_1}\vee \mcal{R}^2_{e_2}\vee
\mcal{R}^3_{e_3}\vee\mcal{R}^4_{e_4}$,
we consider an algorithm
computing a collection of finite set pair
$E_n,F_{n,m}$ by monitoring
$\Phi_{e_i},i\in\{1,2,3,4\}$. Let
$\sigma_i$
denote the string corresponding to
the set $\sigma\cap A_i^c$.

Intuitively, at input
$n$, we monitor
the action of
$\Phi_{e_i}^{Y/\sigma_i}(;1),i\in \{1,2,3,4\}$.
If "very sufficiently"
 many extension of $\sigma$
makes $\Phi_{e_i}(n;1)$ halt,
 then set $E_n$ to be the union of these
output. Denote by $W_{n,1}$ the extension
of $\sigma$ that witness this sufficiency.
This completes the E-round computation at $n$.
To compute $F_{n,m}$, wait for a moment that
there are "sufficiently" many extension of
initial segments \textbf{\emph{in}} $W_{n,1}$
 making $\Phi_{e_i}(n,m;2)$ halt.
If such a moment exists, denote by $F_{n,m}$ the
union of these outputs. This completes the F-round
computation at $n,m$.
If for some $n$ at
some round of computation, there are not sufficiently
many extension that has an output, we apply the
so called type-II extension, which
forces $\Phi_{e_i}$ to be non total for some $i$. If for all
$n$ at all round of computation, there are sufficiently
many extension, then find an $n,m$ at which the output
is "wrong", i.e., $E_n\subseteq \t{E}_{n'},F_{n,m}\subseteq \t{F}_{n'}$
for some $n,m,n'$. We show that we can finitely extend
$\sigma$ to ensure this wrongness.

\begin{algorithm}[H]
\caption{Computing $E_n,F_{n,m}$ by monitoring
$\Phi_{e_i},i\in\{1,2,3,4\}$.}
\begin{algorithmic}
\State The algorithm at input $n,m$ is
as following.

\begin{itemize}
\item E-round:
Let
\begin{align}
P_n =
\bigg\{
\vec{Z}\oplus \vec{Y}=
&Z_1\oplus Z_2\oplus Z_3\oplus Z_4
\oplus Y_1\oplus Y_2\oplus
Y_3\oplus Y_4:\\ \nonumber
&\vec{Z}\text{ and }
\vec{Y}\text{ are 4-partitions of }X-
\{1,2,\cdots,|\sigma|\};\\ \nonumber
&\text{ there exists three different }i_1,
i_2,i_3\in\{1,2,3,4\}
\text{ such that for all }r\in\{1,2,3\},
\text{ all }Z:
\\ \nonumber
&\Phi_{e_{i_r}}^{(Z\cap Z_{i_r}^c\cap Y_{i_r}^c)/\sigma_{i_r}}(n;1)
\uparrow
\vee
\Phi_{e_{i_r}}^{(Z\cap Z_{i_r}^c\cap Y_{i_r}^c)/\sigma_{i_r}}(n;1)
\downarrow\ngtr n\
\bigg\}.
\end{align}
Note that $P_n$ is a $\Pi_1^{0,X}$ class.
If $P_n=\emptyset$,  by compactness argument,
denote by $W_{n,1}$ the witness
that is minimal. i.e.,
 for every pair of 4-partition
 $\vec{Y},\vec{Z}$ of $X
-\{1,2,\cdots,|\sigma|\}$,
there exists  $j_1\ne j_2\in\{1,2,3,4\}$,
$(\rho_1,\rho_2,\rho_3,\rho_4)\in W_{n,1}$ with
$(\forall k) [\rho_k\succeq \sigma_k]$,
$\rho_{j_1}-\sigma_{j_1}\subseteq Z_{j_1}^c\cap
Y_{j_1}^c,
\rho_{j_2}-\sigma_{j_2}\subseteq Z_{j_2}^c\cap
Y_{j_2}^c$
such that ,
$\Phi_{e_{j_1}}^{\rho_{j_1}}(n;1)\downarrow>n\wedge
\Phi_{e_{j_2}}^{\rho_{j_2}}(n;1)\downarrow>n$.

%Let $w_n =
%\max\{|\rho_i|: (\rho_1,\rho_2,\rho_3)\in W_{n,1}, i\leq 3\}$.

Let
$$
E_n = \bigcup\limits_{(\rho_1,\rho_2,\rho_3,\rho_4)
\in W_{n,1}, j\in\{1,2,3,4\}:
\Phi_{e_j}^{\rho_{j}}(n;1)\downarrow>n}
\Phi_{e_j}^{\rho_{j}}(n;1).
$$
Clearly $E_n>n$.

\item F-round:
Let
\begin{align}
Q_{n,m}=\bigg\{
\vec{Y}=&Y_1\oplus Y_2\oplus Y_3\oplus Y_4:\\ \nonumber
&\vec{Y}
\text{ is a 4-partition of } X-\{1,2,\cdots, |\sigma|\} ;
\\ \nonumber
&\text{for all } i\in\{1,2,3,4\},
\text{ all }
(\rho_1,\rho_2,\rho_3,\rho_4 )\in W_{n,1},
\text{all }Z,
\text{ if }\sigma_i\preceq\rho_i\subseteq Y_i^c/\sigma_i,
\text{ then: }
\\ \nonumber
&\hspace{1cm}
\Phi_{e_i}^{\rho_i}(n;1)\downarrow>n\ \Rightarrow\
\Phi_{e_i}^{(Z\cap Y_i^c)/\rho_i}(n,m;2)
\uparrow\vee
\Phi_{e_i}^{(Z\cap Y_i^c)/\rho_i}(n,m;2)\downarrow
\ngtr m
\bigg\}.
\end{align}
Note that
$Q_{n,m}$ is  a $\Pi_1^{0,X}$ class
uniformly in $n,m$.
If
$Q_{n,m}=\emptyset$, by compactness
argument, let
$W_{n,m,2}$ denote the witness.
i.e.,
for all 4-partition $\vec{Y}$ of $X$,
there exists
 $(\rho_1,\rho_2,\rho_3,\rho_4)\in W_{n,m,2}$,
 $j\in\{1,2,3,4\}$
with $(\forall k)
[\rho_k\succeq \sigma_k]$, $
\rho_j\subseteq Y_j^c/\sigma_j $
such that
$\Phi_{e_j}^{\rho_j}(n,m;2)\downarrow
>
m
\wedge
\Phi_{e_j}^{\rho_j}(n;1)
\downarrow >n.
$
In such case, we say F-round at $n$ progress
at part $j$ on $\vec{Y}$.

Let $$
F_{n,m} =
\bigcup\limits_{(\rho_1,\rho_2,\rho_3,\rho_4)
\in W_{n,m,2}; j\in\{1,2,3,4\};
\Phi_{e_j}^{\rho_{j}}(n;1)\downarrow>n\wedge
\Phi_{e_j}^{\rho_{j}}(n,m;2)\downarrow>m}
\Phi_{e_j}^{\rho_{j}}(n,m;2).
$$
Clearly $F_{n,m}>m$.
\end{itemize}

\end{algorithmic}

\end{algorithm}

Now we divide into three cases
and show that in each case we obtain
a valid condition that forces $\mcal{R}_{e_1}^1\vee
\mcal{R}_{e_2}^2\vee \mcal{R}_{c_3}^3\vee\mcal{R}_{e_4}^4$.
\begin{enumerate}
\item Case 1:
for some $n$ $P_n\ne \emptyset$.

\item Case 2:
for all $n,m$ $P_n,Q_{n,m}=\emptyset$.

\item Case 3:
for some $n,m$ $P_n= \emptyset$,
$Q_{n,m}\ne \emptyset$.
\end{enumerate}
Intuitively, in case 1 we apply a simple
type-II extension given by an element of
$P_n$. In case 2 we find some $n,m,n'$ with
$E_n\subseteq \t{E}_{n'},F_{n,m}\subseteq \t{F}_{n'}$
and apply a type-I extension.
Case 3 is a little hard, we show that
we do can apply type-II extension in this case.

\textbf{Case 1}:
Let $\vec{Z}\oplus \vec{Y}$ be an element
of $ P_n$ such that $\EF$ is
$\vec{Z}\oplus \vec{Y}$-\hyper.
Such element must exist since by theorem \ref{TSth2}
$\msf{WKL}$ preserve \propertyL\ and $P_n$ is
a $\Pi_1^{0,X}$ class
with $\EF$ being $X$-\hyper.
Note that at least two of
$Z_i^c\cap Y_i^c,i\in\{1,2,3,4\}$ are infinite.
Suppose, without loss of generality,
$Z_1^c\cap Y_1^c$ and
$ Z_2^c\cap Y_2^c$ are infinite.
By definition of $P_n$,
there exists three different indices $i_1,i_2,i_3\in\{1,2,3,4\}$
 such that
$(\sigma, Z_{i_r}^c\cap Y_{i_r}^c)$
forces $\mcal{R}_{e_{i_r}}^{i_r}$ for all $r\in\{1,2,3\}$.
Therefore either $Z_1^c\cap Y_1^c$
forces $\mcal{R}_{e_1}^1$,
or $Z_2^c\cap Y_2^c$ forces $\mcal{R}_{e_2}^2$.
Suppose $(\sigma, Z_1^c\cap Y_1^c)$
forces $\mcal{R}_{e_1}^1$.
Moreover,
 $(\sigma, Y_{1}^c\cap Z_1^c)\leq
 (\sigma,X)$
is valid
since $Z_{1}^c\cap Y_1^c \leq_T \vec{Z}\oplus\vec{Y}$.

\textbf{Case 2}:
In this case there must exist some
$n,m,n'$ with
$E_n\subseteq \t{E}_{n'}, F_{n,m}\subseteq \t{F}_{n'}\ne\emptyset$
since $\EF$ is $X$-\hyper\ and our computation
 of $E_n,F_{n,m}$
only uses  $X$. For such $n$, since
$\vec{A}\notin Q_{n,m}$,
 then suppose  F-round progress
at part $j$ on $\vec{A}$.
This means there exists a
$(\rho_1,\rho_2,\rho_3,\rho_4)\in W_{n,m,2}$
 with
$\sigma_j\preceq \rho_j\subseteq A_j^c$
 such that
\begin{align}\nonumber
&\Phi_{e_j}^{\rho_j}(n;1)\downarrow
\subseteq E_n\subseteq \t{E}_{n'}
\wedge
\Phi_{e_j}^{\rho_j}(n,m;2)\downarrow\subseteq
F_{n,m}\subseteq \t{F}_{n'}.
\end{align}
 Thus
$(\rho,X)\leq (\sigma,X)$ forces
$\mcal{R}^j_{e_j}$ in a deterministic way,
where $\rho $ is such that
$\rho\cap A_j^c = \rho_j$ and
$\rho\succeq \sigma$.
To see such $\rho$ exists,
let
$\rho$ be the string corresponding to the
set $\sigma\cup \rho_j$.
Then clearly $\rho\cap A_j^c = \rho_j$ since
$\rho_j-\sigma_j
\subseteq A_j^c$ and
 $\sigma\cap A_j^c = \sigma_j$.
 Moreover, $\rho\succeq \sigma$ since
 $\rho_j-\sigma_j> |\sigma|$.

\textbf{Case 3:}
Let $\vec{Z}\in Q_{n,m}$
be such that $\EF$ is $\vec{Z}$-\hyper.
We show that for some $i\in\{1,2,3,4\}$,
$Z_i^c$ is infinite and $(\rho,Z_i^c)\leq (\sigma,X)$
forces $\mcal{R}_{e_i}^i$ for some
$\rho$ determined by an element in $W_{n,1}$.
Since $\vec{Z}
\oplus \vec{A}
\notin P_n$,
there exists $(\rho_1,\rho_2,\rho_3,\rho_4)\in
W_{n,1}$,
$j_1\ne j_2\in\{1,2,3,4\}$
 with $(\forall k)[\rho_k\succeq \sigma_k]$,
  $\rho_{j_1}-\sigma_{j_1}\subseteq
 Z_{j_1}^c\cap A_{j_1}^c,\rho_{j_2}-\sigma_{j_2}\subseteq
 Z_{j_2}^c\cap A_{j_2}^c$ such that
 $\Phi_{e_{j_1}}^{\rho_{j_1}}(n;1)\downarrow>n
 \wedge \Phi_{e_{j_2}}^{\rho_{j_2}}(n;1)\downarrow >n$.
By definition of $Q_{n,m}$,
$(\rho_{j_1},Z_{j_1}^c)$ forces $\mcal{R}_{e_{j_1}}^{j_1}$
and
$(\rho_{j_2},Z_{j_2}^c)$ forces $\mcal{R}_{e_{j_2}}^{j_2}$.
Without loss of generality, suppose
$Z_{j_1}^c$ is infinite (at least three of $Z_1^c,Z_2^c,Z_3^c,Z_4^c$
are infinite).
Let $\rho $ be such a string that
 $\rho\cap A_{j_1}^c =
\rho_{j_1}\wedge \rho\succeq \sigma$.
Therefore $(\rho, Z_{j_1}^c)\leq
(\sigma,X)$ forces
$\mcal{R}_{e_{j_1}}^{j_1}$
is valid.

\subsection{$\msf{LFS}^1$ strongly preserve \propertyL}
\label{TSsec4}
As in section \ref{TSsec3} the result in this section
relativizes therefore it suffices to show that
for any given $\msf{LFS}^1$ instance $c:\omega\rightarrow\omega$,
$c$ admit a free set $G$ such that $\EF$ is $G$-\hyper.
For conceptual
convenience we assume without loss of generality
$c(x)<x$ for all $x\in\omega$.
\subsubsection{Requirements}
We construct an infinite
free set $G$ of $c$ such that $\EF$
is $G$-\hyper.
The requirement we use is for every $e\in\omega$,
\begin{align}
\mcal{R}_e:
(\exists n,m,n')\ \bigg[
&\Phi_e^{G}(n;1)\uparrow\vee
\Phi_e^{G}(n;1)\downarrow \ngtr n
\\ \nonumber
&\vee
\Phi_e^G(n,m;2)\uparrow
\vee\Phi_e^{G}(n,m;2)\downarrow\ngtr m
\\ \nonumber
&\vee
(\Phi_e^G(n;1)\downarrow\subseteq \t{E}_{n'},
\Phi_e^{G}(n,m;2)\downarrow \subseteq
\t{F}_{n'})\ \
\bigg].
\end{align}
The positive requirements are
for every $e\in\omega$,
$$\mcal{P}_{e}: \#G >e.$$
It is plain to see that
if $G $ satisfy all requirements
$\mcal{P}_{e},\mcal{R}_e$ then
$G$ clearly is infinite and
$\EF$ is $G$-\hyper.

\subsubsection{Forcing condition}
The forcing condition we use is still
Mathias condition $(\sigma,X)$.
 The notion of extension and forcing
 are the same as  in subsection \ref{TSsubsec3}.
 In this section,
 a condition $(\sigma,X)$ is \emph{valid }
 if $X$ is infinite, $\EF$
 is $X$-\hyper\ and
 $c(X\cup\sigma)\cap \sigma = \emptyset$
 (recall that we have assumed $c(x)<x$ for all $x$).
 Where $c(X)$ refers to the image of $c$
 on $X$.

 \subsubsection{Framework of proof}

 \begin{lemma}\label{TSlem3}
 For every valid condition
 $(\sigma,X)$ and requirement
 $\mcal{R}_e$,
 there exists a valid condition
 $(\rho,Y)\leq (\sigma,X)$ that forces
 $\mcal{R}_e$.
 \end{lemma}
 The proof is delayed to subsection \ref{TSsubsec4}.
 \begin{lemma}\label{TSlem4}
 For every valid condition,
 there exists a valid condition
 $(\rho,Z)\leq (\sigma,X)$ with
 $\# \rho > \#\sigma$.
 \end{lemma}
\begin{proof}
Consider arbitrary three elements in
$X-\sigma$, namely $x_1,x_2,x_3$.
Consider the following
4-partition of $X$:
\begin{align}
&Y_1 = c^{-1}(x_1)\cap X,\\ \nonumber
&Y_2 = c^{-1}(x_2)\cap X,\\ \nonumber
&Y_3=c^{-1}(x_3)\cap X,\\ \nonumber
&Y_4 = c^{-1}(\omega-\{x_1,x_2,x_3\})\cap X.
\end{align}
Regarding
$Y_1,Y_2,Y_3,Y_4$ as a $\msf{TS}_4^1$ instance.
By strong preservation of \propertyL\ of
$\msf{TS}_4^1$,
suppose  for some
$i\in\{1,2,3,4\}$,
$Y\subseteq Y_i^c\cap X$
is infinite and  $\EF$
is $Y$-\hyper.
Let $\rho$ be the initial segment obtained
by adding $x_i$ into the finite set
$\sigma$. Clearly
$(\rho,Y)\leq (\sigma,X)$ is valid
since $c(Y)\cap \{x_i\} = \emptyset$.

\end{proof}

Clearly lemma \ref{TSlem3},\ref{TSlem4}
guarantee that there exists
 a sequence of forcing condition
$(\sigma_0,X_0)\geq(\sigma_1,X_1)\geq\cdots$, that ultimately forces
all requirements $\mcal{R}_e,\mcal{P}_e$, $e\in\omega$.
Thus these condition's unique common element $G
=\bigcup\limits_{s}\sigma_s$
satisfies all requirements $\mcal{R}_e,\mcal{P}_e,
e\in\omega$.

\subsubsection{Proof of lemma \ref{TSlem3}}
\label{TSsubsec4}
Fix a valid condition $(\sigma,X)$ and
a requirement $\mcal{R}_e$.
The proof is exactly the same as
section \ref{TSsubsec1} with different
combinatorial consideration.
i.e., the two notions, "very sufficient",
"sufficient" are replaced.
Firstly, we consider an algorithm computing  
a collection of finite set pairs.
The failure of this algorithm ensure 
that some valid extension of $(\sigma,X)$ 
forcing $\mcal{R}_e$ exists.

\begin{algorithm}[H]
\caption{Computing $E_n,F_{n,m}$ by monitoring
$\Phi_{e}$.}
\begin{algorithmic}
\State At input $n,m$:

\begin{itemize}
\item E-round:
Let
\begin{align}
P_n = \bigg\{
c_1\oplus c_2:\ \ \
&c_1,c_2 \text{ are }\msf{LFS}^1 \text{ instance with
}
c_1(X\cup \sigma)\cap\sigma,c_2(X\cup\sigma)\cap \sigma = \emptyset;
\\ \nonumber
&\hspace{1cm}
\text{ for any free set }Y
\text{ of both }c_1,c_2,
\text{ with }X/\sigma\supseteq
Y\succeq\sigma\wedge Y-\sigma>n:
\\ \nonumber
&\hspace{5cm}
\Phi_e^{Y}(n;1)\uparrow
\vee
\Phi_e^{Y}(n;1)\downarrow\ngtr n
\bigg\}.
\end{align}

Clearly $P_n$ is a $\Pi_1^{0,X}$ class.
If $P_n=\emptyset$, let
$W_{n,1}$ denote the witness that is minimal. i.e.,
a minimal set of initial segments extending
$\sigma$ such that for every two
$\msf{LFS}^1$ instances $c_1,c_2$,
there exists $\rho\in W_{n,1}$ with
$\rho\subseteq X/\sigma\wedge
\sigma\preceq\rho\wedge\rho-\sigma>n$ and
$\Phi_e^{\rho}(n;1)\downarrow> n$.

Let
$$
E_n = \bigcup\limits_{\rho\in W_{n,1}}
\Phi_e^{\rho}(n;1).
$$
Clearly $E_n>n$.

\item F-round:
Let
\begin{align}
Q_{n,m} = \bigg\{
\t{c}:
\t{c}\text{ is a }&\msf{LFS}^1
 \text{ instance with }\t{c}(X\cup\sigma)\cap \sigma = \emptyset;
  \\ \nonumber
 &\hspace{1cm}
  \text{ for any  }\rho\in W_{n,1},
  \text{ any free set }Y\text{ of }
 \t{c} \text{ with }
  \rho\preceq Y\subseteq X/\rho
  \wedge Y-\sigma>n:
  \\ \nonumber
 &\hspace{5cm}
 \Phi_e^{Y}(n,m;2)\uparrow
\vee
\Phi_e^{Y}(n,m;2)\downarrow\ngtr m
\bigg\}.
\end{align}

Clearly $Q_{n,m}$ is a $\Pi_1^{0,X}$
class uniformly in $n,m$.
If $Q_{n,m}=\emptyset$, let
$W_{n,m,2}$ denote the minimal witness. i.e.,
a set of initial segments extending
$\sigma$ such that for every
$\msf{LFS}^1$ instance $\t{c}$,
there exists $\rho\in W_{n,m,2}$ with
$\rho\subseteq X/\sigma\wedge \sigma\preceq\rho
\wedge \rho-\sigma>n$ and
$\Phi_e^{\rho}(n;1)\downarrow
>n\wedge \Phi_e^{\rho}(n,m;2)\downarrow
> m$.

Let $$
F_{n,m} = \bigcup\limits_{\rho\in W_{n,m,2}}
\Phi_e^{\rho}(n,m;2).
$$
Clearly $F_{n,m}>m$.

\end{itemize}

\end{algorithmic}

\end{algorithm}
Now we divide into three cases.
\begin{enumerate}
\item Case 1: for some
$n$ $P_n\ne\emptyset$;

\item Case 2: for
all but finitely many $n$:
 $(\forall m)\ [P_n,Q_{n,m}=\emptyset]$.

\item Case 3: for infinitely many
$n$:
$(\exists m)[
P_n= \emptyset,
Q_{n,m}\ne\emptyset]$.
\end{enumerate}

\textbf{Case 1}:
Let $c_1\oplus c_2\in P_n$
be such that $\EF$
is $c_1\oplus c_2$-
\hyper. Such path in $P_n$ is guaranteed
by theorem \ref{TSth2}: $\msf{WKL}$ preserve
\propertyL.
As shown in the following claim \ref{TSclaim1},
any $\msf{LFS}^1$ instance compute an infinite
 free set of
itself. Let
$\sigma\preceq Y\subseteq X$ be an infinite free set for
 both $c_1,c_2$
computed by $c_1\oplus c_2$
(such $Y$ exists since $c_1(X)\cap \sigma,c_2(X)\cap \sigma=
\emptyset$).
 Then clearly
$(\sigma, Y)\leq (\sigma,X)$ forces
$\mcal{R}_e$. Because
any set $\sigma\preceq Z\subseteq Y/\sigma$ is
a free set for both $c_1,c_2$, so
$\Phi_e^{Z}(n;1)\uparrow
\vee
\Phi_e^{Z}(n;1)\downarrow\ngtr n$.
Condition $(\sigma,Y)$ is also valid since
$c(Y)\subseteq c(X)$ and $c(X)\cap \sigma=\emptyset$.
\begin{claim}\label{TSclaim1}
Every $\msf{LFS}^1$ instance, $c$,
 compute an infinite free set of
itself.
\end{claim}
\begin{proof}
If $\# c^{-1}(x) = \infty$ for some
$x$. Then $c^{-1}(x)$ is free for $c$ and
is computable in $c$.
If $\# c^{-1}(x)<\infty$ for all $x$,
simply add more and more
elements while keep being free
for $c$.

\end{proof}

\textbf{Case 2}:
Since $\EF$ is \hyper, there exists
infinitely many $n,m,n'$ such that
$E_n\subseteq \t{E}_{n'},
F_{n,m}\subseteq \t{F}_{n'}$.
Let $(n_1,m_1,n_1'), (n_2,m_2,n_2'),( n_3,m_3,n_3'),
(n_4,m_4,n_4')
$ be four of them
with $(\forall k\leq 3)\ [
n_{k+1}> \max\{x:x\in \rho, \rho\in W_{n_k,m_k,2}\}
]$.
Since $c\notin Q_{n,m}$, then there exists
$\rho_j\in W_{n_j,m_j,2},j\in\{1,2,3,4\}$
being a finite free set of $c$
with $
\sigma\preceq \rho_j\subseteq X/\sigma$
such that
$$\Phi_e^{\rho_j}(n_j;1)\downarrow\subseteq
E_{n_j}\subseteq
\t{E}_{n_j'},\Phi_e^{\rho_j}(n_j,m_j;2)\downarrow
\subseteq F_{n_j,m_j}\subseteq \t{F}_{n_j'}
.$$
So $(\rho_j,X)$ forces $\mcal{R}_e$ deterministically
for all $j\in\{1,2,3,4\}$. Now we show that some valid 
extension of $(\rho_j,X)$ exists for some $j$.
Note that $\rho_j-\sigma,j\in\{1,2,3,4\}$ are mutually disjoint
since for every $\tau_j\in W_{n_j,m_j,2},
\tau_{j+1}\in W_{n_{j+1},m_{j+1},2}$,
$\tau_j-\sigma<\tau_{j+1}-\sigma$.
Thus consider the following 4-partition of
$X$,
\begin{align}\nonumber
&Y_1 = c^{-1}(\rho_1-\sigma)\cap X,\\ \nonumber
&Y_2 = c^{-1}(\rho_2-\sigma)\cap X,\\ \nonumber
&Y_3=c^{-1}(\rho_3-\sigma)\cap X,\\ \nonumber
&Y_4 = c^{-1}\big(\ (\omega-\rho_{1}-\rho_{2}-\rho_3)
\cup \sigma\big)\cap X.
\end{align}
Taking $Y_1,Y_2,Y_3,Y_4$
as  a $\msf{TS}_4^1$
instance, by strong preservation of \propertyL\ 
of $\msf{TS}_4^1$,
there exists a $i\in\{1,2,3,4\}$,
 a $Z\subseteq Y_i^c\cap X$ being infinite
such that $\EF$ is $Z$-\hyper.
But $c(Z)\cap \rho_i = \emptyset$
(recall that $c^{-1}(X\cup \sigma)\cap \sigma = \emptyset$
since $(\sigma,X)$ is valid).
Therefore $(\rho_i,Z)\leq (\sigma,X)$ is valid
and $(\rho_i,Z)$ forces
$\mcal{R}_e$ deterministically.

\textbf{Case 3}:
Let $n_1,n_2,n_3,n_4$ be such  that
$P_{n_j}=\emptyset\wedge Q_{n_j,m_j}\ne\emptyset\wedge$
$n_{j+1}>\max\{x:x\in \rho,\rho\in W_{n_j,1}\}$
for all $j\in\{1,2,3,4\}$.
Such $n_1,n_2,n_3,n_4$ exists since for infinitely many
$n$: there exists $m$ with $P_n= \emptyset$,
$Q_{n,m}\ne\emptyset$.
Let
$\t{c}_j\in Q_{n_j,m_j},j\in\{1,2,3,4\}$ be such that
 $\EF$ is $\t{c}_1\oplus \t{c}_2\oplus \t{c}_3\oplus \t{c}_4$-\hyper.
Since $c\oplus \t{c}_j\notin P_{n_j}$, there exists
$\rho_j\in W_{n_j,1}$ being free for both
$c, \t{c}_j$ with
$\rho_j\subseteq X/\sigma\wedge \sigma\preceq\rho_j\wedge
\rho_j-\sigma>n_j$ and
$\Phi_e^{\rho_j}(n;1)\downarrow> n$.
Let $Y\leq_T \t{c}_1\oplus \t{c}_2\oplus \t{c}_3
\oplus \t{c}_4$
 be an infinite free set for all
$\t{c}_j,j\in\{1,2,3,4\}$ with $(\forall j\in\{1,2,3,4\})
\ [Y\cap \rho_j=\emptyset]$.
Clearly,
$(\rho_j,Y)$ forces $\mcal{R}_e$ for all $j\in\{1,2,3,4\}$
by definition of $Q_{n,m}$.
We apply again the strong preservation of
$\msf{TS}_4^1$ to obtain a valid condition
$(\rho_i,Z)\leq (\rho_i,Y)$.
Consider the 4-partition of $Y$:
$Y_1 = c^{-1}(\rho_{1}-\sigma)\cap Y,
Y_2 = c^{-1}(\rho_{2}-\sigma)\cap Y,
Y_3=c^{-1}(\rho_3-\sigma),
Y_4 = c^{-1}\big(\sigma\cup
 (\omega-\rho_{1}-\rho_{2}-\rho_3)\ \big)\cap Y$.
Suppose
$Z\subseteq Y_i^c\cap Y$ is infinite and
$\EF$ is $Z$-\hyper.
Then $(\rho_i,Z)\leq (\rho_i,Y)$ is clearly valid
since $c(Z)\cap \rho_i = \emptyset$.

\subsection{$\msf{UFS}^2$ preserve \propertyL}
\label{TSsec5}
We transform a computable
$\msf{UFS}^2$ instance $c$ into a
tree $T\subseteq h(\cdot)^{<\omega}$
 of width (bushiness) $n\mapsto h(n)-n^2$ such that
any path through $T$ computes an infinite free set
of $c$.
Here $h(\cdot):\omega\rightarrow\omega$
 is a computable order that is sufficiently
 large (dominating any quadratic function)
  to guarantee that  trees of bushyness
  $h$ are
 "combinatorially weak".

 \begin{definition}
 A tree $T$ is \emph{pruned } if every
 $\rho\in T$ extends to a path.
 A tree $T\subseteq h(\cdot)^{<\omega}$
 is of \emph{bushiness} $k(\cdot):\omega\rightarrow\omega$
 iff for every $\rho\in T$ that is not a leaf of $T$,
  $\rho$ has at least
 $k(|\rho|+1)$ many successor in $T$.
 A tree $T\subseteq h(\cdot)^{<\omega}$
 is of bushiness $k(\cdot):\omega\rightarrow\omega$
 \emph{after } $n^{th}$ level
 if every $\rho\in T $ with $|\rho|\geq n$ that is not a leaf,
 has at least $k(|\rho|+1)$ many successor in $T$.
 \end{definition}
Note that a pruned tree $T$ is of bushiness $k(\cdot)$
if every $\rho$ has at least $k(|\rho|)$ many successor that
can  be extend to a path through $T$.
  We firstly demonstrate the transformation
 of $\msf{UFS}^2$ into a sufficiently bushy tree
 in lemma \ref{TSlem8}. Then we focus on strong
 preservation of \propertyL\ of a tree instance that
 is sufficiently bushy.

\begin{lemma}\label{TSlem8}
Given computable order
$h$ dominating function
$n\mapsto 2n^2$, given a $\msf{UFS}^2$ instance
$c$,
there exists a pruned tree
$T\subseteq h^{<\omega}$ of bushiness
$n\mapsto h(n)-n^2$ such that every
path through $T$ compute an infinite free set
of $c$.

\end{lemma}
\begin{proof}
Fix a computable one-one function from
$h(\cdot)^{<\omega}$ to $\omega$. Therefore
in the proof of this lemma,
we regard each $\rho\in h(\cdot)^{<\omega}$
as an integer.
For any set $Z$, let $$H_{Z} = \{x:\{x\}\cup Z
\text{ is free for }c \}.$$
We inductively define $T\subseteq h(\cdot)^{<\omega}$
such that $H_{\{\tau:\tau\preceq\rho\}}$
is infinite for all $\rho\in T$ (this automatically guarantees
that for any $\rho\in T$,
$\{\tau:\tau\preceq\rho\}$
is itself free for $c$).
The first
level of $T$ is simply $h^{\leq 1}$.
Clearly $H_{\{\tau:\tau\preceq \rho\}}$
is infinite for any $\rho\in 2^1\cap T$.
Suppose the $n^{th}$ level of $T$ is defined.
For any $\rho$, consider
the finite set $
\big\{\alpha:\alpha \text{ is a successor of }\rho
\big\} =
\{\alpha_1,\cdots,\alpha_{h(n+1)}\}$.
Consider
the set
$$\t{H}_\rho =
\{\alpha:
\alpha\text{ is a successor of }\rho
\text{ in }h^{<\omega},
 H_{\{\alpha\}\cup \{\tau:\tau\preceq\rho\}}
\text{ is finite.}\}$$

Note that
$\#\t{H}_\rho\leq n+n(n-1)/2\leq n^2$.
To see this, note that there are at most
$n(n-1)/2$ many successors
$\alpha_1,\cdots,\alpha_m$
of $\rho$ with
$\alpha_i\in c\big(\ [\{\tau:\tau\preceq \rho\}]^2\ \big)$.
For a
successor $\alpha\notin c\big(\ [\{\tau:\tau\preceq \rho\}]^2\ \big)$
of $\rho$,
for any
$x\in H_{\{\tau:\tau\preceq\rho\}}-
c\big(\ [\{\tau:\tau\preceq \alpha\}]^2\ \big)
$ with
$x> \max\{\tau:\tau\preceq \alpha\}$,
$\{x,\alpha\}\cup\{\tau:\tau\preceq \rho\}$ being
non-free for $c$
means  $(\exists y\in \{\tau:\tau\preceq \rho\})
\big[\ c(\{y,x\}) = \alpha \big]$.
In another word,
for a successor
$\alpha\notin c\big(\ [\{\tau:\tau\preceq \rho\}]^2\ \big)$
of $\rho$,
$H_{\{\alpha\}\cup\{\tau:\tau\preceq\rho\}}$
being finite means for all but finitely many $x\in
H_{\{\tau:\tau\preceq\rho\}}$,
$(\exists  y\in \{\tau:\tau\preceq \rho\})
[\ c(\{x,y\}) = \alpha\ ].$
i.e., $\alpha$ "occupies" some predecessor of
$\rho$ for almost all the time. But $c$ is a single valued
function. So at each time a predecessor of $\rho$
can be occupied by at most one descendent of $\rho$.
Thus there are at most $|\rho|=n$ such successors
that occupies some predecessor of $\rho$ all the time.

By definition of $\t{H}_\rho$,
for any successor $\alpha\notin \t{H}_\rho$ of $\rho$,
$H_{\{\tau:\tau\preceq \rho\}\cup\{\alpha\} }$
is infinite.
The $(n+1)^{th}$ level 
of $T$ consists of successors of 
$\rho$ that is not in $\t{H}_\rho$.
 This accomplish the definition of
$T$. Clearly
$T$ is of bushiness $
h(n+1)-n^2\geq h(n+1)-(n+1)^2$
since at each level $n+1$, at most
$n^2$ elements from $h^{<\omega}$
are deleted.
Moreover, for any path $G$ through $T$,
 $G$ as a set of integer
is itself free for $c$ since
any initial segment of $G$ is free.

\end{proof}

Now fix an arbitrary computable order
 $h:\omega\rightarrow\omega$
  that dominate any quadratic function.
It remains
to prove that 
a tree of bushiness $n\mapsto h(n)-n^2$
strongly preserve \propertyL.
\begin{theorem}\label{TSth5}
Given any set $C$ with
$\EF$ being $C$-\hyper,
for any pruned tree $\t{T}\subseteq h^{<\omega}$ of
bushiness $n\mapsto h(n)-n^2$,
there exists a path $G$ through $\t{T}$
such that $\EF$ is $G\oplus C$-\hyper.
\end{theorem}
The rest of this section is devoted to prove
theorem \ref{TSth5}. Since our results
clearly relativize, we assume $C = \emptyset$.
Fix a pruned tree $\t{T}$ given
in theorem \ref{TSth5}.
\subsubsection{Requirements}
The requirements are for every $e\in\omega$,
\begin{align}
\mcal{R}_e:
(\exists n,n',m)\ \bigg[
&\Phi_e^{G}(n;1)\uparrow\vee
\Phi_e^{G}(n;1)\downarrow\ngtr n
\\ \nonumber
&\vee
\Phi_e^{G}(n,m;2)\uparrow\vee
\Phi_e^{G}(n,m;2)\downarrow\ngtr m
\\ \nonumber
&\vee
(\Phi_e^{G}(n;1)\downarrow
\subseteq\t{E}_{n'},
\Phi_e^{G}(n,m;2)\downarrow\subseteq
\t{F}_{n'})
\ \
\bigg].\\ \nonumber
\mcal{P}_e:
|G| >e.&
\end{align}

\subsubsection{Forcing condition}
In this section, a forcing condition
is a triple
$(\sigma, T,r)$ where $\sigma\in h^{<\omega}$
, $T\subseteq h^{<\omega}$ is a pruned tree and
$r$ is a positive integer.
A forcing condition $(\sigma,T,r)$ is \emph{valid}
iff $[\sigma]^{\preceq}\cap [T]\ne\emptyset$,
$T$ is of bushiness $h(n)-rn^2$ after $|\sigma|$ and
$h(n)> 3rn^2$ for all $n\geq |\sigma|$.
 Note that $T$ can be of arbitrary
computational power.
$(\rho,T',r')$ extends $(\sigma,T,r)$ iff
$\rho\succeq \sigma $ and $[\rho]^\preceq
\cap [T']\subseteq [\sigma]^\preceq\cap [T]$.
The forcing condition
$(\sigma,T)$ is also regarded as a collection of
sets $[T]\cap [\sigma]^\preceq$.
Thus the notion of extension of a condition
and forcing follows automatically. %

\subsubsection{Framework of proof}
\begin{lemma}\label{TSlem6}
For every valid condition $(\sigma, T,r)$,
there exists a valid condition $(\rho,T',r')
\leq (\sigma,T,r)$ such that
$(\rho,T',r')$ forces requirement $\mcal{R}_e$.
\end{lemma}
The proof is delayed to section \ref{TSsubsec5}.
Meeting positive requirements is
trivial for tree forcing condition.

\begin{lemma}\label{TSlem7}
For every  valid condition $(\sigma, T,r)$,
there exists a valid condition $(\rho,T,r)
\leq (\sigma,T,r)$ such that
$(\rho,T,r)$ forces requirement $\mcal{P}_e$.
\end{lemma}
\begin{proof}
Simply extend $\sigma$ to a level
higher than $e$.
Such extension must exist
since $[\sigma]^\preceq \cap [T]\ne\emptyset$.
\end{proof}
We set the first condition
$d_0$ to be $(\varepsilon,\t{T},1)$ which is
obviously valid.
Clearly lemma \ref{TSlem6},\ref{TSlem7}
guarantee a sequence of valid conditions
$(\varepsilon,\t{T},1)\geq (\sigma^1,T^1,r_2)\geq \cdots $
that ultimately
forces every requirement
$\mcal{R}_e,\mcal{P}_e$.
Thus $G=\bigcup\limits_{s} \sigma^s$ is the
desired path through $\t{T}$ that forces all requirements.

\subsubsection{Proof of lemma \ref{TSlem7}}
\label{TSsubsec5}
Fix a valid forcing condition $(\sigma,T,r)$
and a requirement $\mcal{R}_e$.
Consider the following algorithm computing
a collection of finite sets $E_n,F_{n,m},n,m\in\omega$.
\begin{algorithm}[H]
\caption{Computing $E_n,F_{n,m}$ by monitoring
$\Phi_{e}$.}
\begin{algorithmic}
\State At input $n,m$:
\begin{itemize}
\item E-round:
Let
\begin{align}
P_n=\bigg\{
T_1\oplus T_2:
T_1,T_2\subseteq h^{<\omega}
 &\text{ are pruned tree of bushiness }n\mapsto h(n)-rn^2,
 \text{ with }[\sigma]^\preceq\cap [T_1]\cap [T_2]
 \ne\emptyset.
 \\ \nonumber
 &\text{ Moreover, }
 \text{for any Y}\in [T_1]\cap [T_2]\cap [\sigma]^\preceq:
 \Phi_e^{Y}(n;1)\uparrow
\vee
\Phi_e^{Y}(n;1)\downarrow\ngtr n.
\bigg\}
\end{align}

Note that $P_n$ is a $\Pi_1^{0}$ class.
If $P_n = \emptyset$, let
$W_{n,1}$ be the minimal witness,
i.e., for any pruned tree
$T_1,T_2\subseteq h^{<\omega}
 $ of bushiness $n\mapsto h(n)-rn^2$,
there exists
$Y\in [T_1]\cap [T_2]\cap [\sigma]^\preceq$,
 $\rho\in W_{n,1}$
 with $Y\succ\rho\succeq \sigma$ such that
$\Phi_e^{\rho}(n;1)\downarrow> n$.

Let $$
E_n = \bigcup\limits_{\rho\in W_{n,1}}
\Phi_e^\rho(n,1).
$$
Clearly $E_n>n$.

\item
Let
\begin{align}
Q_{n,m} = \bigg\{
T':
T'\subseteq h^{<\omega}
 &\text{ is a pruned tree of bushiness }
 n\mapsto h(n)-rn^2
 \text{ with }
 [\sigma]^\preceq\cap [T']
 \ne\emptyset.
 \\ \nonumber
 &\text{ For any }\rho\in W_{n,1},
 \text{ any }Y\in[T']\cap[\sigma]^\preceq
 \text{ with }Y\succ \rho:
 \\ \nonumber
 &\hspace{1cm}
 \Phi_e^{Y}(n,m;2)\uparrow
\vee
\Phi_e^{Y}(n,m;2)\downarrow\ngtr n.
\bigg\}
\end{align}

Note that $Q_{n,m}$ is a $\Pi_1^0$ class.
If $Q_{n,m}=\emptyset$, let
$W_{n,m,2}$ be the minimal witness. i.e.,
for any pruned tree $T'\subseteq
h^{<\omega}$ of bushiness
$n\mapsto h(n)-rn^2$,
there exists $Y\in[T']\cap[\sigma]^\preceq $,
 $\rho\in W_{n,m,2},\rho\preceq Y$ such
that
$\Phi_e^{\rho}(n,m;2)\downarrow> m
\wedge
\Phi_e^{\rho}(n;1)\downarrow>n$.

Set $$
F_{n,m} = \bigcup\limits_{\rho\in W_{n,m,2}}
\Phi_e^{\rho}(n,m;2).
$$
Clearly $F_{n,m}>m$.
\end{itemize}
\end{algorithmic}
\end{algorithm}

Now we divide into three cases.
\begin{enumerate}

\item Case 1:
for some $n$, $P_n\ne \emptyset$.

\item Case 2:
for all $n,m$, $P_n,Q_{n,m}=\emptyset$.

\item Case 3:
for some $n,m$, $P_n= \emptyset$,
$Q_{n,m}\ne \emptyset$.

\end{enumerate}

\textbf{Case 1}:
Let $T_1\oplus T_2\in P_n$
be arbitrary. Consider
the tree $T' = T_1\cap T_2\cap T$.
The key point is that
$T'$ is of bushiness
$n\mapsto h(n)-3rn^2>0$
after $|\sigma|$. Therefore,
$T'$ is pruned. Moreover,
by definition of $P_n$,
$(\sigma,T',3r)\leq (\sigma,T,r)$ clearly forces
$\mcal{R}_e$. Now simply extend
$\sigma$ to some $\rho$
such that
$[\rho]^\preceq\cap [T']
\ne\emptyset $ and
$h(n)>9r n^2$ for all
$n\geq |\rho|+1$.
Such $\rho$ must exist since
$ T'$ is of bushiness
$n\mapsto h(n)-3rn^2$ and
$h(n)>3rn^2$ for all $n\geq |\sigma|$
(also recall that $h(\cdot)$ is monotonically
nondecreasing and dominate
any quadratic function so
$h(n)\geq 9rn^2$ for all
$n\geq |\rho|$ can also be
satisfied).
Thus
$(\rho,T',3r)\leq (\sigma,T,r)$ is valid.

\textbf{Case 2}:
There must exist some $n,n'$ with
$E_n\subseteq \t{E}_{n'},
F_{n,m}\subseteq \t{F}_{n'}$.
Since $T\notin Q_{n,m}$, there exists $Y\in [T]
\cap [\sigma]^\preceq$ and
$\rho\in W_{n,m,2}$ with
$\rho\preceq Y$, such that
$\Phi_e^{\rho}(n;1)\downarrow> n
\wedge
\Phi_e^{\rho}(n,m;2)\downarrow>
n$
(such $Y$ must exist since
$ T$ is of bushiness $n\mapsto h(n)-rn^2$
after $|\sigma|$ and $h(n)>3rn^2$ for
all $n\geq |\sigma|$, so $[T]\ne\emptyset$).
Clearly $(\rho, T, r)\leq (\sigma, T,r)$
forces $\mcal{R}_e$ deterministically since
$\Phi_e^{\rho}(n;1)
\subseteq E_n\subseteq \t{E}_{n'},
\Phi_e^\rho(n,m;2)\subseteq
F_{n,m}\subseteq \t{F}_{n'}$.
Meanwhile,
$(\rho,T,r)$ is clearly valid
since $Y\in [\rho]^\preceq\cap [T]\ne\emptyset$.

\textbf{Case 3}:
For $Q_{n,m}\ne\emptyset$,
let $T'\in [Q_{n,m}]$ be arbitrary.
Since $T\oplus T'\notin P_n$,
then there exists $\rho\in W_{n,1}$
with $ [T]\cap [T']\cap [\rho]^\preceq\ne
\emptyset\wedge \rho\succeq \sigma$.
For any
$Y\in [T']\cap [\rho]^\preceq$,
by definition of $Q_{n,m}$,
 $\Phi_e^{Y}(n,m;2)\uparrow
\vee
\Phi_e^{Y}(n,m;2)\downarrow\ngtr m
$.
Thus $(\rho, T')$ forces
$\mcal{R}_e$.
Meanwhile $T'\cap T$ is of bushiness
$n\mapsto h(n)-2rn^2$ after $|\rho|$, so
$T'\cap T$ is pruned. Furthermore,
$[\rho]^\preceq\cap [T']\cap [T]
\ne\emptyset$. Therefore $\rho$
can be extended to some $\alpha$, such that
$[\alpha]^\preceq
\cap [T'\cap T]
\ne\emptyset$ and
$ h(n)>6rn^2$ for all $n\geq |\alpha|$.
Thus $(\alpha,T'\cap T,2r)\leq (\sigma,T,r)$ is  a valid
condition that forces $\mcal{R}_e$.
